# Supplementary material for: Anytime Replanning of Robot Coverage Paths for Partially Unknown Environments
Source: arXiv:2311.17837 source file (2024-06-07)
Supplement: Supplementary file 1 [file Appendix.tex]

\begin{align}
    \label{eq:new-milp-2}
    \text{RANKMILP}(\boldsymbol{\Bar{y}_h}, \boldsymbol{\Bar{y}_v}, t_h) & = \\
    & \min_{\boldsymbol{x_h}, \boldsymbol{x_v}} m\\
    \text{s.t.} 
    & \quad a \leq m_O \label{eq:violating-constraint}\\ 
    % & \quad s \geq 0\\
    \nonumber & \quad \text{Eqs. (\ref{eq:c1-new}), (\ref{eq:c2-new}), (\ref{eq:c3}), (\ref{eq:c4})}
\end{align}

}

Unlike the MILP from OARP, a direct relaxation of RANKMILP does not necessarily yield integral solutions. This is due to the addition of the constraint Eq. (\ref{eq:violating-constraint}) which violates TUM property exhibited by the constraints otherwise.

\begin{proposition}
The constraints of RANKMILP are not necessarily TUM.
\end{proposition}
\begin{proof}
We prove this by showing a counter-example where the addition of constraint Eq. (\ref{eq:violating-constraint}) violates. For simplicity of the proof, let us assume that $\hat{t}_\text{r}$ and $t_h$ are 1. We start by following a similar structure as in our proof in \cite{rameshOptimalPartitioningNonConvex2022a} and write the constraints in Standard Equality Form (SEF) by adding slack variables as follows:
\begin{align*}
\begin{bmatrix}
A_L^T & A_R^T
\end{bmatrix}^T\boldsymbol{x_h} - \boldsymbol{y_h} + \boldsymbol{z_1} = \boldsymbol{0}\\
\begin{bmatrix}
A_T^T & A_B^T
\end{bmatrix}^T\boldsymbol{x_v} - \boldsymbol{y_v} + \boldsymbol{z_2} = \boldsymbol{0} \\
\boldsymbol{x_h} + \boldsymbol{x_v} = \boldsymbol{1}\\
(\boldsymbol{1} - \boldsymbol{\Bar{y}_h})^T \boldsymbol{y_h} + (\boldsymbol{1} - \boldsymbol{\Bar{y}_v})^T \boldsymbol{y_v} - s + z_3 = 1 \label{eq:violating-constraint-eq} \\
\boldsymbol{x_h}, \boldsymbol{x_v}, \boldsymbol{y_h}, \boldsymbol{y_v}, s, \boldsymbol{z_1}, \boldsymbol{z_2}, z_3 \geq \boldsymbol{0}
\end{align*}
Let $A_H = \begin{bmatrix}A_L^T & A_R^T\end{bmatrix}^T$ and $A_V =\begin{bmatrix}A_T^T & A_B^T\end{bmatrix}^T$. Note that $A_H$ and $A_V$ are NAI matrices themselves as each row signifies a directed edge in the graph, with a -1 for the source grid cell (outgoing), a +1 for the sink grid cell (incoming), and 0s otherwise \cite{nemhauserIntegerCombinatorialOptimization1999}. Also, let $\boldsymbol{\Bar{0}}$ be the matrix of zeros and $I$ be the identity matrix. The constraints are now of the form $A\boldsymbol{x} = \boldsymbol{b}$, where
\begin{align*}
A & = \begin{bmatrix} A_H & \boldsymbol{\Bar{0}} & -I & \boldsymbol{\Bar{0}} & \boldsymbol{\Bar{0}} & I & \boldsymbol{\Bar{0}} & \boldsymbol{\Bar{0}}\\
\boldsymbol{\Bar{0}} & A_V & \boldsymbol{\Bar{0}} & -I & \boldsymbol{\Bar{0}} & \boldsymbol{\Bar{0}} & I & \boldsymbol{\Bar{0}} \\
I & I & \boldsymbol{\Bar{0}} & \boldsymbol{\Bar{0}} & \boldsymbol{\Bar{0}} & \boldsymbol{\Bar{0}} & \boldsymbol{\Bar{0}} & \boldsymbol{\Bar{0}} \\
0 & 0 & (\boldsymbol{1} - \boldsymbol{\Bar{y}_h})^T & (\boldsymbol{1} - \boldsymbol{\Bar{y}_v})^T & 1 & 0 & 0 & 1
\end{bmatrix}
\end{align*}
\begin{align*}
\boldsymbol{b} & = \begin{bmatrix} \boldsymbol{0}^T & \boldsymbol{0}^T & \boldsymbol{1}^T & 1
\end{bmatrix}^T,
\end{align*}
\begin{align*}
\boldsymbol{x} & = \begin{bmatrix}
\boldsymbol{x_h}^T &
\boldsymbol{x_v}^T &
\boldsymbol{y_h}^T &
\boldsymbol{y_v}^T &
s &
\boldsymbol{z_1}^T &
\boldsymbol{z_2}^T &
z_3
\end{bmatrix}^T.
\end{align*}

\begin{figure}
    \centering
    \includegraphics[width=0.7\linewidth]{Assets/Not TUM example.png}
    \caption{Counterexample to show that the constraints of the new problem are not TU.}
    \label{fig:counterexample}
\end{figure}

Consider the simple example shown in Fig. \ref{fig:counterexample}, where the environment consists of only two grid cells connected horizontally. The corresponding $A_H$ and $A_V$ are as follows:
\begin{align}
    A_H = \begin{bmatrix} 1 & 0 \\
-1 & 1 \\
1 & -1 \\
0 & 1 \end{bmatrix} & \quad
    A_V = \begin{bmatrix} 1 & 0 \\ 1 & 0 \\ 0 & 1 \\ 0 & 1 \end{bmatrix}.
\end{align}
Consider the example where the initial path covers both grid cells horizontally, i.e. $\boldsymbol{\Bar{y}_h}^T = [1, 0, 0, 1]$ and $\boldsymbol{\Bar{y}_v}^T = [0, 0, 0, 0]$. Using these, we can extract a square submatrix $S$ that has a determinant of $2$ as follows:
\begin{align}
S = \begin{bmatrix} 1 & 0 & -1 & 0 \\
-1 & 1 & 0 & 0 \\
0 & 1 & 0 & -1 \\
0 & 0 & 1 & 1 \end{bmatrix}.
\end{align}
This violates the property of a TUM matrix, as the determinant of any square submatrix must be in $\{0, +1, -1\}$. Therefore, the constraints of this LP are not necessarily TUM and may not give integral solutions.
\end{proof}
